# Supplementary material for: The impact of one-way streets on the asymmetry of the shortest commuting routes
Source: arXiv:2111.07434 ancillary file (2021-11-14)
Supplement: Supplementary file 1 [file SM.pdf]

# Supplemental Material - The impact of one-way streets on the asymmetry of the shortest commuting routes

Hygor P. M. Melo,[1,*] Diogo P. Mota,[1] José S. Andrade Jr.,[2] and Nuno A. M. Araújo[1,3,†]

[1] *Centro de Física Teórica e Computacional, Faculdade de Ciências, Universidade de Lisboa, 1749-016 Lisboa, Portugal*

[2] *Departamento de Física, Universidade Federal do Ceará, 60451-970, Fortaleza, Ceará, Brazil*

[3] *Departamento de Física, Faculdade de Ciências, Universidade de Lisboa, 1749-016 Lisboa, Portugal*

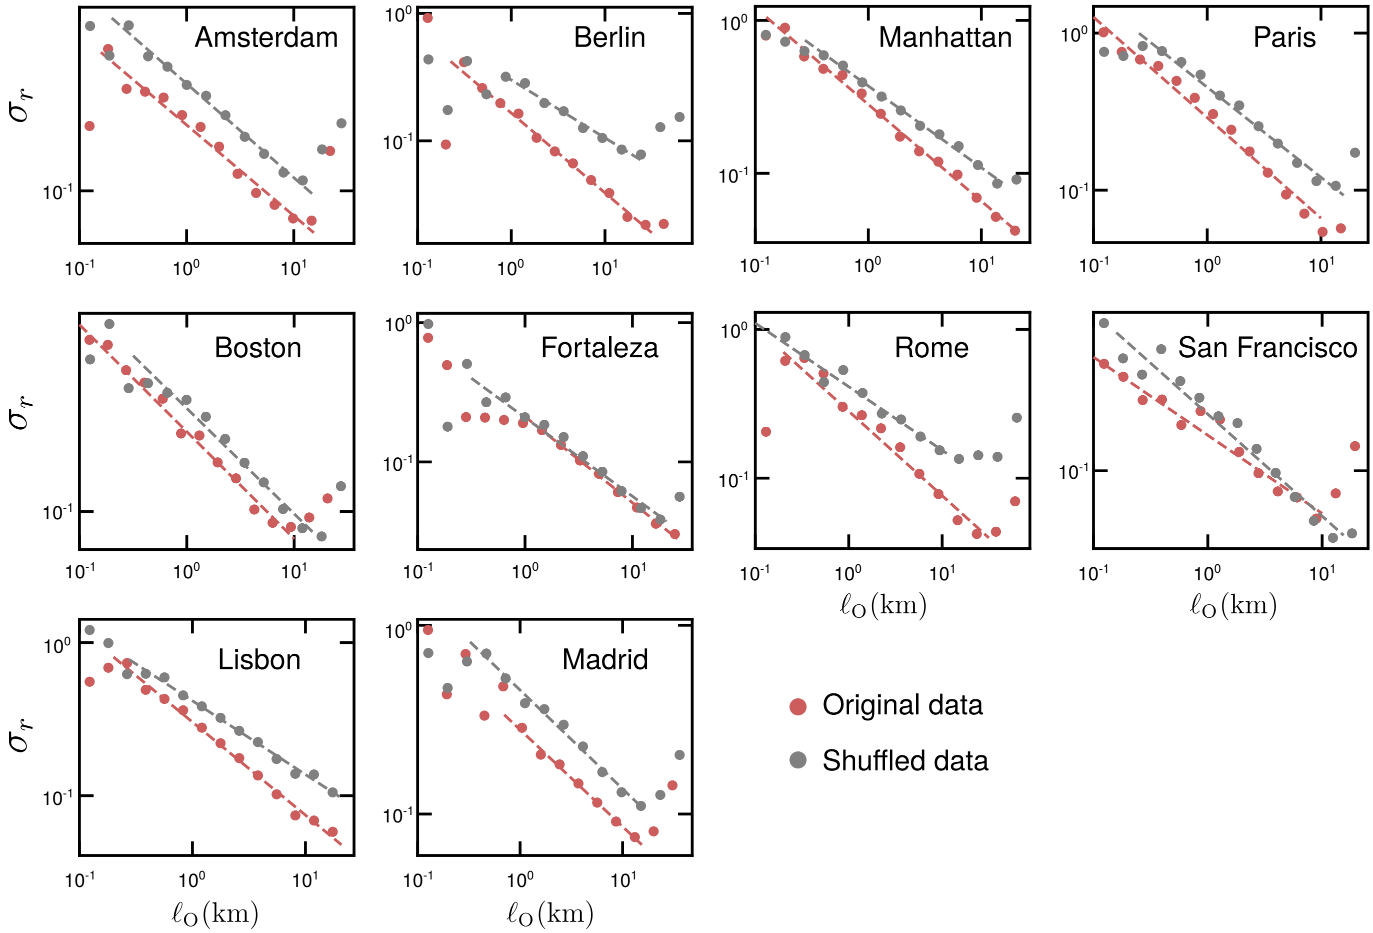


FIG. 1. **Shuffling and fluctuations, $\sigma_r$, as a function of $\ell_0$ for all cities.** We show that the fluctuations of $r$ decay as a power law for all cities, $\sigma_r \sim \ell_O^{-\beta}$. The gray circles are for the original data while the red circles are for the shuffled street network. The dashed gray lines are the power-law fit for all cities with corresponding $\beta$ exponents: Amsterdam ($0.47 \pm 0.03$), Berlin ($0.63 \pm 0.03$), Manhattan ($0.63 \pm 0.02$), Paris ($0.64 \pm 0.03$), Boston ($0.53 \pm 0.03$), Fortaleza ($0.62 \pm 0.02$), Rome ($0.57 \pm 0.04$), San Francisco ($0.40 \pm 0.04$), Lisbon ($0.61 \pm 0.02$), and Madrid ($0.51 \pm 0.02$). After shuffling the position of one-way streets, we see that all $\beta$ exponents are close to 0.5: Amsterdam ($0.48 \pm 0.02$), Berlin ($0.45 \pm 0.03$), Manhattan ($0.53 \pm 0.02$), Paris ($0.57 \pm 0.03$), Boston ($0.52 \pm 0.03$), Fortaleza ($0.57 \pm 0.03$), Rome ($0.43 \pm 0.04$), San Francisco ($0.53 \pm 0.04$), Lisbon ($0.48 \pm 0.02$), and Madrid ($0.52 \pm 0.03$). The exponents were calculated by averaging over the least-squares fit of 100 bootstrapping samples and the error is one standard deviation.

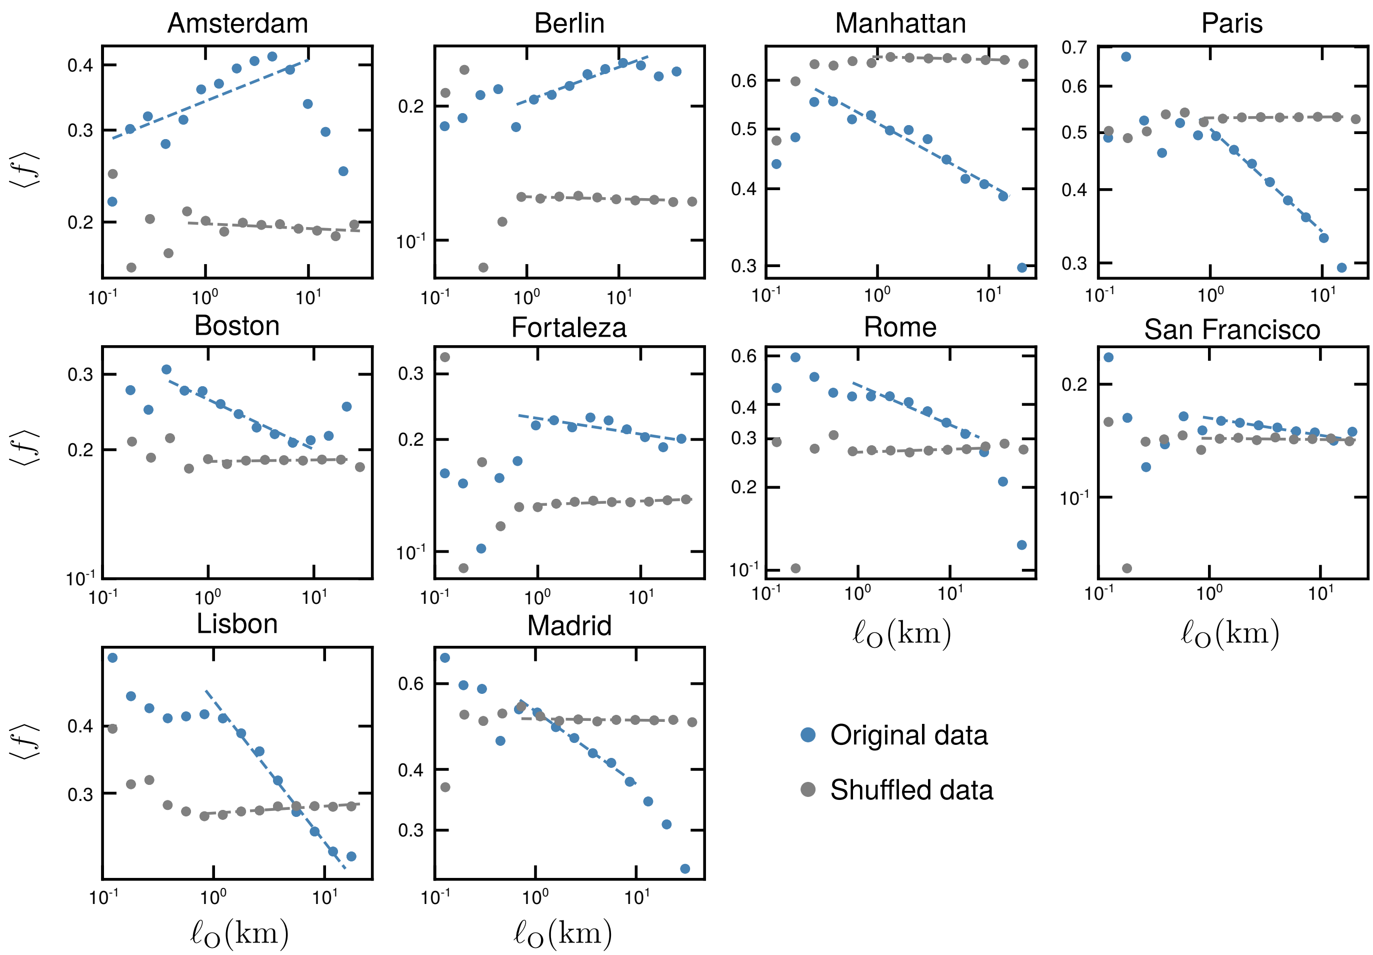


FIG. 2. **Shuffling and fraction of one-way streets in the shortest routes, $\langle f \rangle_{\ell_O}$, as a function of $\ell_0$ for all cities.** We show that the fraction of one-way $\langle f \rangle_{\ell_O}$ is a power-law function of $\ell_0$ for all cities, $\langle f \rangle_{\ell_O} \sim \ell_O^{-\alpha}$. The gray circles are for the original data while the blue circles are the average fraction of one-way streets in the shortest routes for the shuffled street network. The dashed gray lines are the power-law fit for all cities with the corresponding $\alpha$ exponents: Amsterdam ($-0.08 \pm 0.03$), Berlin ($-0.08 \pm 0.01$), Manhattan ($0.10 \pm 0.01$), Paris ($0.18 \pm 0.01$), Boston ($0.12 \pm 0.01$), Fortaleza ($0.04 \pm 0.01$), Rome ($0.14 \pm 0.02$), San Francisco ($0.05 \pm 0.01$), Lisbon ($0.26 \pm 0.01$), and Madrid ($0.15 \pm 0.01$). After shuffling the position of one-way streets, we see that all $\alpha$ exponents are close to 0.0: Amsterdam ($0.009 \pm 0.007$), Berlin ($0.005 \pm 0.008$), Manhattan ($0.004 \pm 0.001$), Paris ($-0.002 \pm 0.002$), Boston ($-0.004 \pm 0.004$), Fortaleza ($-0.010 \pm 0.005$), Rome ($-0.011 \pm 0.006$), San Francisco ($0.003 \pm 0.005$), Lisbon ($-0.013 \pm 0.004$), and Madrid ($0.003 \pm 0.003$). The exponents were calculated by averaging over the least-squares fit of 100 bootstrapping samples and the error is one standard deviation.

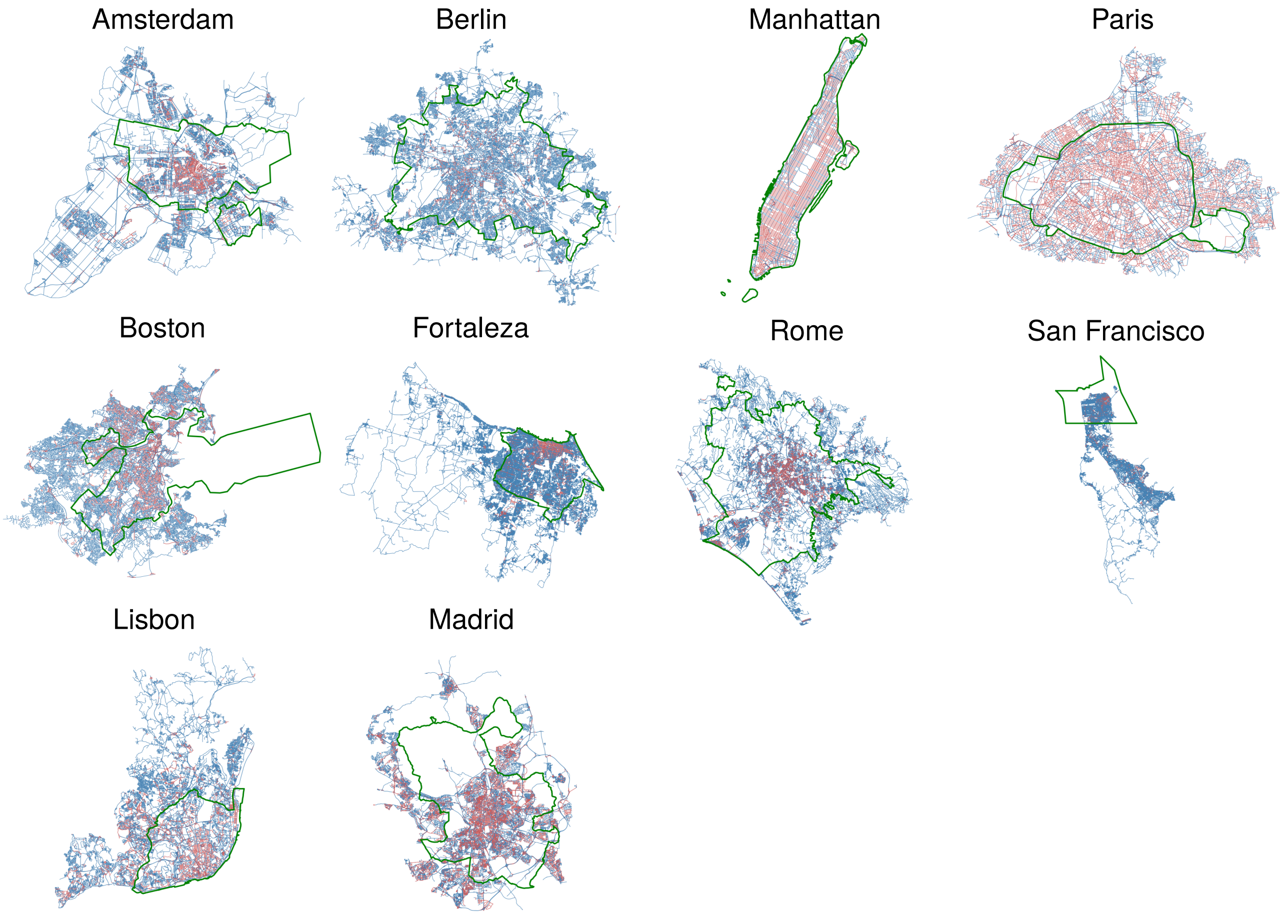


FIG. 3. **Street map of all cities.** Street map for all the ten cities, where one-way segments are in red and two-way segments are in blue. To reduce finite size effects in the calculation of the shortest routes, we included the neighboring cities. The main street network is delimited by the green polygon and it is where the origin-destination pairs of points are selected.
